# Supplementary material for: Topological Foundations of Reinforcement Learning
Source: arXiv:2410.03706 source file (2024-09-25)
Supplement: Supplementary file 1 [file appendixA.tex]

\chapter{Some additional data}
\label{app:additionalData}
% We number appendices as in the main file, A, B, C.
% The appendice has title, do not include "Appendix" in the chapter name.
% You need permission from Prof. Mama to have appendices
% Why is it necessary? Does it add value?
